# Supplementary material for: Chemical reaction motifs driving non-equilibrium behaviors in phase separating materials
Source: arXiv:2207.10135 source file (2022-12-02)
Supplement: Supplementary file 1 [file SupplementaryInformation.pdf]

# Supplementary Information for chemical reaction motifs driving non-equilibrium behaviors in phase separating materials

Dino Osmanović[1,*] and Elisa Franco[1,2]

[1]Department of Mechanical and Aerospace Engineering,
University of California, Los Angeles, Los Angeles 90095, CA, USA

[2]Department of Bioengineering, University of California, Los Angeles, Los Angeles 90095, CA, USA

(Dated: November 29, 2022)

## I. CREATION OF RANDOM CHEMICAL REACTION NETWORKS

We discuss how a random chemical reaction network is generated, interested readers can consult reference [1] for further details.

A Chemical Reaction can be defined through two objects, a stoichiometric matrix $\underline{S}$, which tells us what reactants each substrate is constituted of and a reaction graph (the nodes of which are the substrates), which specifies which substrates interconvert between one another. The tuple $(N_r, S_u, R_e)$ specifies the number of reactants, substrates, and reactions, respectively.

Introducing a matrix $\underline{Z}$ where each column is a set of integers corresponding to the substrate, e.g., when there are 4 reactants and the substrate is $z_1 + z_2$ the column will be $(1, 1, 0, 0)$and each row is a unique substrate. The Stoichiometric matrix is given by:

$$\underline{S} = \underline{Z}.\underline{B} \tag{1}$$

where $\underline{B}$ is the incidence matrix of the reaction graph.

We introduce the weighted incidence graph $\underline{A}$, where each non-zero element $A_{ij}$ corresponds to some rate of reaction of substrate $i$ to substrate $j$. Further introducing a matrix $\underline{L} = \underline{\Delta} - \underline{A}$ where $\Delta$ is a diagonal matrix where the $ith$ element is equal to the total of column $i$ of matrix $\underline{A}$, the mass action kinetics of such a network for the vector of reactant concentrations $\mathbf{x}$ will be given by:

$$\dot{\mathbf{x}} = -\underline{Z}\underline{L}\mathrm{Exp}(\underline{Z}^T \mathrm{Ln}(\mathbf{x})) \tag{2}$$

where the functions $\mathrm{Exp}, \mathrm{Ln}$ are elementwise applications of $\exp, \ln$ to a vector $\mathbf{x}$

To generate a random reaction network, we go through the following process:

- Every possible substrate of the $n$ reactants is generated. This is performed through generating all tuples of length $n$ from the vector $(0, 1, 2)$. In words, we focus only on substrates of the form $az_1 + \ldots \rightarrow$ where a is at most 2.
- From this substrate list, we select those which have a stochiometric total of at least 1 and at most 3. The former condition means there is no spontaneous creation of chemical and the latter condition limits reactions to the form $2z_1 + z_2$ or $z_1 + z_2 + z_3$ etc. This leaves us with a set of substrate matrices $\{\underline{Z}\}$
- We generate incidence graphs of the reactions by considering the entire set of $S_u \times S_u$ matrices $\{\underline{A}\}$ which have $2R$ non-zero elements corresponding to interconversion between substrates. For example if substrates $S_1$ and $S_2$ interconvert, and substrates $S_3$ and $S_4$ interconvert, we would have the following reaction matrix:

$$\begin{pmatrix} 0 & k_1 & 0 & 0 \\ k_2 & 0 & 0 & 0 \\ 0 & 0 & 0 & k_3 \\ 0 & 0 & k_4 & 0 \end{pmatrix} \tag{3}$$

  where the $k_i$ are the rates

* osmanovic.dino@gmail.com

- From this set $\{\underline{Z}\}, \{\underline{A}\}$ we analyze every unique pair from each set. An algorithm identifies degenerate matrices and removes them from the set.
- Every reaction network is analyzed to make sure that it obeys conservation laws on the total mass, this is to make sure there is no spontaneous creation or destruction of material. This can be done through analysis of the null space of the matrix $\underline{S}$, and ensuring that every reactant participates in some conservation law. Each reaction is also parsed separately and analyzed for whether it locally conserves mass. Randomly generated CRNs that violate these conditions are excluded from analysis.
- The algebraic system corresponding to the mass action kinetics is solved for its stationary points $\mathbf{x}_0$ using the Solve routine of *Mathematica*. This is the point around which the linear stability analysis is performed.
- The Jacobian around the stationary point is generated for the chemical dynamics and for the diffusive dynamics. The dispersion curve is generated, and then features of the dispersion curve are analyzed in terms of their real or imaginary components (for dynamics), or the total number of crossing points, the points where the dispersion crosses zero (for size).
- For full simulation of the reaction diffusion equation, we have written code which parses the output of the above and generates a file that can be read by a separate reaction diffusion solver we have coded, that can take an arbitrary chemical reaction network as an input and generate the corresponding equations to be solved numerically. This is discussed in the next section.

### A. Generation of a Jacobian from a CRN and calculating the score

To illustrate how a Jacobian can be generated from a chemical reaction network, we shall work through an example. Let us use the example CRN from the maintext given by:

$$\mathrm{z}_1 \underset{k_2}{\overset{k_1}{\rightleftharpoons}} \mathrm{z}_2 \tag{4}$$

$$2\,\mathrm{z}_2 \underset{k_4}{\overset{k_3}{\rightleftharpoons}} \mathrm{z}_1 + \mathrm{z}_2 \tag{5}$$

This set of chemical reactions leads to the following mass-action kinetics:

$$\frac{\mathrm{d}z_1}{\mathrm{d}t} = k_4 z_2^2 + k_1 z_2 - k_3 z_1 z_2 - k_2 z_1 \tag{6}$$

$$\frac{\mathrm{d}z_2}{\mathrm{d}t} = -k_4 z_2^2 - k_1 z_2 + k_3 z_1 z_2 + k_2 z_1 \tag{7}$$

This has a stable fixed point at $z_1 = (-k_1 z_2 - k_4 z_2^2)/(-k_2 - k_3 z_2)$. We can calculate the Jacobian of these equations around this fixed point, which is given by:

$$J_R = \begin{pmatrix} -k_3 z_2 - k_2 & 2k_4 z_2 - \frac{k_3\left(-k_4 z_2^2 - k_1 z_2\right)}{-k_3 z_2 - k_2} + k_1 \\ k_3 z_2 + k_2 & -2k_4 z_2 + \frac{k_3\left(-k_4 z_2^2 - k_1 z_2\right)}{-k_3 z_2 - k_2} - k_1 \end{pmatrix} \tag{8}$$

Then, by inserting random values of $k_1, k_2, \ldots, x_2$ etc we can calculate the structure score of this CRN.

## II. PHASE SEPARATING SYSTEM IN THE ABSENCE OF CHEMICAL REACTIONS

In the main text, we have confined our analysis to situations where the system has both reactions and conserved interactions. It is reasonable to pose the question what can be achieved, in terms of spatial organization, in the absence of any chemical reactions (we note that in the absence of any conserved interactions, each spatial point behaves independently, and therefore the system would just correspond to mass action kinetics). While the potential scope of such a question is large, we limit ourselves to analysis of the model we presented in the main text without chemistry, given in the equations (1) and (2) there.

One way to make progress on such a problem is via the analysis of the linear dispersion relation over many different choices of the interaction parameters $\boldsymbol{\epsilon}$ and seeing whether there exists a set of parameters over which the growth rate is *negative* at small values of $|\mathbf{k}|$. As was discussed in the main text, microphase separation is associated with negative growth rates at small values of $|\mathbf{k}|$. In figure Sa we observe that no choice of parameters yields negative growth rates at small values of $|\mathbf{k}|$. We therefore conclude that in our model, the presence of chemistry is necessary for microphase separation.

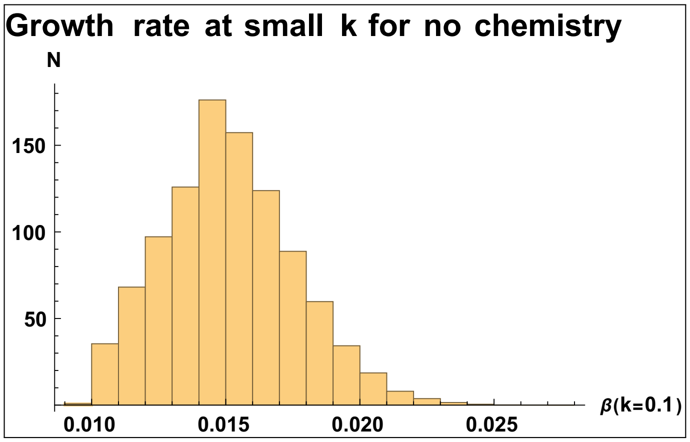


FIG. Sa. Histogram of the value of the growth rate at small values of $|\mathbf{k}|$ for the phase separating functional defined in the main paper in the absence of any chemical reactions, over many different choices of interaction parameters. The growth rate is always positive, suggesting that microphase separation in this system only arises with the introduction of chemistry.

## III. NUMERICAL SOLUTIONS OF EQUATIONS

When it is required, we solve the full equation via a Fourier scheme. This is achieved in the following way:

- The entire specification of the system is passed as an input to a reaction-diffusion program we wrote, this constructs the equations

$$\dot{\mathbf{c}} = \mathbf{I}(\mathbf{c}(\mathbf{x},t)) + \mathbf{R}(\mathbf{c}(\mathbf{x},t)) \tag{9}$$

  seen in the main text

- The linear and non-linear terms of $\mathbf{I}$ are split $\mathbf{I}(\mathbf{c}(\mathbf{x},t)) = \mathbf{I}_L(\mathbf{c}(\mathbf{x},t)) + \mathbf{I}_{NL}(\mathbf{c}(\mathbf{x},t))$

- The update equations can be iterated by the following rearrangement

$$\mathbf{c}^{n+1} - \Delta t I_L(\mathbf{c}^{n+1}) = \mathbf{c}^n + \Delta t(\mathbf{I}_{NL}(\mathbf{c}(\mathbf{x},t)) + \mathbf{R}(\mathbf{c}(\mathbf{x},t))) \tag{10}$$

  As the left hand side of this equation is linear, the equation can be represented as a matrix equation $\mathbf{M}.\mathbf{c}^{n+1}$. Inversion of $M$ then gives us the time evolution over the set of fields $\mathbf{c}$

- It is easiest to do this in Fourier space to treat the spatial derivatives. We therefore iterate our equations firstly by calculating all the weights in real space, Fourier converting them using fast fourier transform methods, applying the update rule equation 10 and then converting back to real space

The Fourier transforms are performed with the aid of the FFTW C++ Library. All other aspects of the code were written by D.O. The full repository is available at https://github.com/osmanovicdino/FieldTheory

## IV. EXAMPLE MODELS

In figure 5. of the main text, we showed the results of different CRNS coupled to phase separating systems. The chemical reaction network associated to each state is listed below:

A.

$$\mathrm{z}_1 + \mathrm{z}_3 + \mathrm{z}_4 \underset{k_2}{\overset{k_1}{\rightleftharpoons}} 2\,\mathrm{z}_3 \tag{11}$$

$$2\,\mathrm{z}_4 \underset{k_4}{\overset{k_3}{\rightleftharpoons}} \mathrm{z}_3 \tag{12}$$

B.

$$\mathrm{z}_1 + \mathrm{z}_3 \underset{k_2}{\overset{k_1}{\rightleftharpoons}} \mathrm{z}_3 + 2\,\mathrm{z}_4 \tag{13}$$

$$2\,\mathrm{z}_1 + \mathrm{z}_4 \underset{k_4}{\overset{k_3}{\rightleftharpoons}} \mathrm{z}_2 + \mathrm{z}_3 + \mathrm{z}_4 \tag{14}$$

C.

$$\mathrm{z}_1 + \mathrm{z}_2 + \mathrm{z}_3 \underset{k_2}{\overset{k_1}{\rightleftharpoons}} 2\,\mathrm{z}_2 \tag{15}$$

$$\mathrm{z}_2 + \mathrm{z}_3 \underset{k_4}{\overset{k_3}{\rightleftharpoons}} \mathrm{z}_2 + \mathrm{z}_4 \tag{16}$$

D.

$$\mathrm{z}_1 + \mathrm{z}_3 \underset{k_2}{\overset{k_1}{\rightleftharpoons}} 2\,\mathrm{z}_2 + \mathrm{z}_4 \tag{17}$$

$$2\,\mathrm{z}_1 + \mathrm{z}_2 \underset{k_4}{\overset{k_3}{\rightleftharpoons}} \mathrm{z}_3 \tag{18}$$

E.

$$\mathrm{z}_2 + 2\,\mathrm{z}_3 \underset{k_2}{\overset{k_1}{\rightleftharpoons}} \mathrm{z}_1 + 2\,\mathrm{z}_4 \tag{19}$$

$$2\,\mathrm{z}_1 + \mathrm{z}_4 \underset{k_4}{\overset{k_3}{\rightleftharpoons}} 2\,\mathrm{z}_4 \tag{20}$$

F.

$$\mathrm{z}_1 + 2\,\mathrm{z}_2 \underset{k_2}{\overset{k_1}{\rightleftharpoons}} 2\,\mathrm{z}_3 + \mathrm{z}_4 \tag{21}$$

$$\mathrm{z}_1 + \mathrm{z}_2 + \mathrm{z}_4 \underset{k_4}{\overset{k_3}{\rightleftharpoons}} \mathrm{z}_2 + \mathrm{z}_3 + \mathrm{z}_4 \tag{22}$$

Table I shows all of the parameters associated with each of these simulations:

| Chemistry | $k_1$ | $k_2$ | $k_3$ | $k_4$ | $\epsilon_{12}$ | $\epsilon_{13}$ | $\epsilon_{14}$ | $\epsilon_{23}$ | $\epsilon_{24}$ | $\epsilon_{34}$ | $x_1(0)$ | $x_2(0)$ | $x_3(0)$ | $x_4(0)$ |
|---|---|---|---|---|---|---|---|---|---|---|---|---|---|---|
| A | 0.892462 | 0.580214 | 0.964577 | 1.85727 | −0.782956 | −0.218338 | 0.24518 | 0.175683 | −0.946703 | 0.247882 | 0.29633 | 0.48462 | 0.400028 | 0.877635 |
| B | 1.11787 | 1.73653 | 1.60228 | 0.528507 | −0.694135 | 0.225322 | −0.384434 | −0.264477 | −0.888883 | −0.991619 | 0.557349 | 1.3343 | 0.705813 | 0.598988 |
| C | 1.91221 | 0.585953 | 1.30007 | 1.04792 | 0.975771 | 0.717489 | 0.0754955 | 0.0208708 | 0.199087 | −0.397392 | 0.231439 | 0.42905 | 0.568065 | 0.704749 |
| D | 1.38827 | 0.316002 | 1.32923 | 1.94859 | 0.194255 | 0.771281 | 0.421889 | 0.784968 | −0.639263 | 0.564329 | 1.14865 | 0.488903 | 0.440023 | 9.28971 |
| E | 1.10084 | 0.761341 | 1.74671 | 0.442901 | −0.960903 | −0.85777 | 0.760997 | 0.377102 | −0.21782 | −0.983576 | 0.206281 | 0.0041252 | 0.986887 | 0.167816 |
| F | 0.527847 | 1.3201 | 1.9928 | 1.6836 | 0.739195 | 0.368704 | 0.247701 | 0.691255 | −0.373446 | −0.526562 | 0.723848 | 0.239717 | 0.856786 | 0.0226568 |

TABLE I. Parameters for the above chemistries.

Where every simulation has the same parameters $\gamma = 0.4$,$D = 1$,$c_0 = 0.2$ and $c_1 = 0.8$.

[1] A. Van Der Schaft, S. Rao, and B. Jayawardhana, On the Mathematical Structure of Balanced Chemical Reaction Networks Governed by Mass Action Kinetics, (2011), arXiv:1110.6078v1.
